# Supplementary material for: Asymptotic analysis of covariance parameter estimation for Gaussian processes in the misspecified case
Source: arXiv:1412.1926 source file (2015-11-12)
Supplement: Supplementary file 1 [file bachoc15asymptotic_supplement.pdf]

# Supplementary material for: Asymptotic analysis of covariance parameter estimation for Gaussian processes in the misspecified case

François Bachoc\*  
Institut de Mathématiques de Toulouse

November 10, 2015

## Abstract

We restate some context elements of the manuscript “Asymptotic analysis of covariance parameter estimation for Gaussian processes in the misspecified case”. Then, we restate and prove technical lemmas that are used there.

## 1 Context elements

**Condition 1.1.** For all  $n \in \mathbb{N}^*$ , the observation points  $X_1, \dots, X_n$  are random and follow independently the uniform distribution on  $[0, n^{1/d}]^d$ . The three variables  $Y$ ,  $(X_1, \dots, X_n)$  and  $\epsilon$  are mutually independent.

**Condition 1.2.** The covariance function  $K_0$  is stationary and continuous on  $\mathbb{R}^d$ . There exists  $C_0 < +\infty$  so that for  $t \in \mathbb{R}^d$ ,

$$|K_0(t)| \leq \frac{C_0}{1 + |t|^{d+1}}.$$

**Condition 1.3.** For all  $\theta \in \Theta$ , the covariance function  $K_\theta$  is stationary. For all fixed  $t \in \mathbb{R}^d$ ,  $K_\theta(t)$  is  $p+1$  times continuously differentiable with respect to  $\theta$ . For all  $i_1, \dots, i_p \in \mathbb{N}$  so that  $i_1 + \dots + i_p \leq p+1$ , there exists  $A_{i_1, \dots, i_p} < +\infty$  so that for all  $t \in \mathbb{R}^d$ ,  $\theta \in \Theta$ ,

$$\left| \frac{\partial^{i_1}}{\partial \theta_1^{i_1}} \dots \frac{\partial^{i_p}}{\partial \theta_p^{i_p}} K_\theta(t) \right| \leq \frac{A_{i_1, \dots, i_p}}{1 + |t|^{d+1}}.$$

There exists a constant  $C_{inf} > 0$  so that, for any  $\theta \in \Theta$ ,  $\delta_\theta \geq C_{inf}$ . Furthermore,  $\delta_\theta$  is  $p+1$  times continuously differentiable with respect to  $\theta$ . For all  $i_1, \dots, i_p \in \mathbb{N}$  so that  $i_1 + \dots + i_p \leq p+1$ , there exists  $B_{i_1, \dots, i_p} < +\infty$  so that for all  $\theta \in \Theta$ ,

$$\left| \frac{\partial^{i_1}}{\partial \theta_1^{i_1}} \dots \frac{\partial^{i_p}}{\partial \theta_p^{i_p}} \delta_\theta \right| \leq B_{i_1, \dots, i_p}.$$

In all this supplementary material, it is assumed that Conditions 1.1, 1.2 and 1.3 hold.

**Definition 1.4.** Consider a fixed  $\theta \in \Theta$ . Consider two functions of  $n$ :  $n_2(n) \in \mathbb{N}^*$  and  $\Delta(n) \geq 0$ , that we write  $n_2$  and  $\Delta$  for simplicity, so that, for any  $n \in \mathbb{N}^*$ ,  $n_2$  can be written  $n_2 = N_2^d$ , with  $N_2 \in \mathbb{N}^*$ , and so that  $n = n_2 \Delta$ . Let, for  $i = 1, \dots, N_2 - 1$ ,  $c_i = [((i-1)/N_2)n^{1/d}, (i/N_2)n^{1/d}]$ . Let  $c_{N_2} = [(N_2 - 1)/N_2 n^{1/d}, n^{1/d}]$ . Let, for  $x \in [0, n^{1/d}]$ ,  $i(x)$  be the unique  $i \in \{1, \dots, N_2\}$

---

\*The research leading to this paper was partly carried out when the author was affiliated to the University of Vienna.

so that  $x \in c_i$ . Let, for  $t = (t_1, \dots, t_d)^t \in [0, n^{1/d}]^d$ ,  $C(t) = \prod_{j=1}^d c_{i(t_j)}$ . Define the non-stationary covariance function  $\tilde{K}_\theta(t_1, t_2) = K_\theta(t_1, t_2) \mathbf{1}_{C(t_1)=C(t_2)}$ . Define  $\tilde{R}_\theta$ ,  $\tilde{R}_{i,\theta}$ ,  $\tilde{r}_{i,\theta}$ ,  $\tilde{y}_{i,\theta}$ ,  $\tilde{C}V_\theta$  similarly to  $R_\theta$ ,  $R_{i,\theta}$ ,  $r_{i,\theta}$ ,  $\hat{y}_{i,\theta}$ ,  $CV_\theta$  but with  $K_\theta$  replaced by  $\tilde{K}_\theta$ . Furthermore, let us write the  $n_2$  aforementioned sets of the form  $\prod_{j=1}^d c_{i_j}$ , for  $i_1, \dots, i_d \in \{1, \dots, N_2\}$ , as the sets  $C_1, \dots, C_{n_2}$ . [The specific one-to-one correspondence we use between  $\{1, \dots, N_2\}^d$  and  $\{1, \dots, n_2\}$  is of no interest. Note that this one-to-one correspondence depends on  $n$ . The sets  $C_1, \dots, C_{n_2}$  also depend of  $n$ , but we drop this dependence in the notation for simplicity.]

Let  $N_i$  be the random number of observation points in  $C_i$  and let  $X^i$  be the random  $N_i$ -tuple obtained from  $X$  by keeping only the observation points that are in  $C_i$  and by preserving the order of the indices in  $X$ . Let  $y^i$  be the column vector of size  $N_i$ , composed by the components  $y_j$  of  $y$  for which  $X_j$  is in  $C_i$  (preserving the order of indexes). Let  $\bar{R}_{i,\theta}$  and  $\bar{R}_{i,0}$  be the covariance matrices, under  $(K_\theta, \delta_\theta)$  and  $(K_0, \delta_0)$ , of  $y^i$ , given  $X$ .

Finally, for  $1 \leq i, j \leq n_2$ , let  $v_i$  and  $w_j$  be two  $N_i \times 1$  and  $N_j \times 1$  vectors and  $M^{ij}$  be a  $N_i \times N_j$  matrix. Then we use the convention that, when  $N_i = 0$ ,  $|M^{ij}| = ||M^{ij}|| = 0$ ,  $||v_i|| = |v_i| = 0$  and  $v_i^t M^{ij} w_j = 0$ . Furthermore, if  $i = j$  and  $M^{ii}$  is invertible when  $N_i \geq 1$ , we use the convention that  $v_i^t (M^{ii})^{-1} w_i = 0$  when  $N_i = 0$ . [These conventions enable to write equalities or inequalities involving matrices and vectors of size  $N_i$ ,  $N_j$  or  $N_i \times N_j$ , that hold regardless of whether  $N_i$  or  $N_j$  are zero or not. As can be checked along the proofs involving Definition 1.4, these relations boil down to trivial relations (e.g.  $0 = 0$ ) when  $N_i = 0$  or  $N_j = 0$ . This way of proceeding considerably simplifies the exposition in these proofs.]

## 2 Technical results

**Lemma 2.1.** Consider a fixed number  $n$  of observation points. Consider a function  $f_\theta(X, y)$  that is  $p$  times continuously differentiable w.r.t  $\theta$  for any  $X, y$  and so that, for  $i_1 + \dots + i_p \leq p$ ,

$$\sup_{\theta} |(\partial^{i_1}/\partial \theta_1^{i_1}) \dots (\partial^{i_p}/\partial \theta_p^{i_p}) f_\theta(X, y)|$$

has finite mean value w.r.t  $X$  and  $y$ . Then, there exists a constant  $C_{sup}$  (depending only of  $\Theta$ ) so that

$$\mathbb{E} \left( \sup_{\theta \in \Theta} |f_\theta(X, y)| \right) \leq C_{sup} \sum_{i_1 + \dots + i_p \leq p} \int_{\Theta} \mathbb{E} \left( \left| \frac{\partial^{i_1}}{\partial \theta_1^{i_1}} \dots \frac{\partial^{i_p}}{\partial \theta_p^{i_p}} f_\theta(X, y) \right| \right) d\theta.$$

**Lemma 2.2.** There exists a finite constant  $C_{sup}$  so that, for any  $a, b \in \mathbb{R}^d$ ,

$$\int_{\mathbb{R}^d} \frac{1}{1 + |a - c|^{d+1}} \frac{1}{1 + |b - c|^{d+1}} dc \leq C_{sup} \frac{1}{1 + |a - b|^{d+1}}.$$

**Lemma 2.3.** Let  $0 < C_{inf} \leq C_{sup} < \infty$  be fixed independently of  $n$ . Let  $s_n$  be a function of  $n$  so that  $s_n \in \mathbb{N}^*$  and  $C_{inf}n \leq s_n \leq C_{sup}n$ . Consider  $s_n$  observation points  $\bar{X}_1, \dots, \bar{X}_{s_n}$ , independent and uniformly distributed on  $[0, n^{1/d}]^d$ . Let  $A_1, \dots, A_k$  be  $k$  sequences of  $s_n \times s_n$  random matrices so that, for  $l = 1, \dots, k$ ,  $(A_l)_{i,j}$  depends only on  $\bar{X}_i$  and  $\bar{X}_j$  and satisfies  $|(A_l)_{i,j}| \leq 1/(1 + |\bar{X}_i - \bar{X}_j|^{d+1})$ . Then  $\mathbb{E}_X (|A_1 \dots A_k|^2)$  is bounded w.r.t.  $n$ .

**Lemma 2.4.** The supremum over  $n$ ,  $\theta$  and  $X$  of the eigenvalues of  $R_\theta^{-1}$ ,  $R_{1,\theta}^{-1}$ ,  $\text{diag}(R_\theta^{-1})$ ,  $\text{diag}(R_{1,\theta}^{-1})$ ,  $\text{diag}(R_\theta^{-1})^{-1}$  and  $\text{diag}(R_{1,\theta}^{-1})^{-1}$  is smaller than a constant  $C_{sup} < +\infty$ .

**Lemma 2.5.** Lemma 2.4 also holds when  $K_\theta$  is replaced by  $\tilde{K}_\theta$  of Definition 1.4.

**Lemma 2.6.** Lemma 2.4 also holds when  $R_\theta$  is replaced by  $\bar{R}_{k,\theta}$  of Definition 1.4.

**Lemma 2.7.** Let  $k \in \mathbb{N}$ . Let  $A_{1,\theta}, \dots, A_{k,\theta}$  be  $k$  sequences of symmetric random matrices (functions of  $X$  and  $\theta$ ) so that, for any  $m \in \mathbb{N}$ ,  $a_1, \dots, a_m \in \{1, \dots, k\}$ ,  $\sup_{\theta \in \Theta} \mathbb{E}_X |A_{a_1,\theta} \dots A_{a_m,\theta}|^2$  is bounded (w.r.t  $n$ ). Let  $B_{1,\theta}, \dots, B_{k+1,\theta}$  be  $k+1$  sequences of random symmetric non-negative

matrices (functions of  $X$  and  $\theta$ ) so that  $\sup_{\theta} \|B_{1,\theta}\|, \dots, \sup_{\theta} \|B_{k+1,\theta}\|$  are bounded (w.r.t  $n$  and  $X$ ). Then

$$\sup_{\theta \in \Theta} \mathbb{E}_X |B_{1,\theta} A_{1,\theta} B_{2,\theta} \dots B_{k,\theta} A_{k,\theta} B_{k+1,\theta}|^2$$

is bounded w.r.t  $n$ .

**Lemma 2.8.** Consider a fixed  $\theta \in \Theta$ . With the notation of Definition 1.4, we have, when  $n_2 = o(n)$ ,

$$\mathbb{E} \left( \left| (R_{1,\theta} - \tilde{R}_{1,\theta})^2 \right|^2 \right) \rightarrow_{n \rightarrow \infty} 0.$$

**Lemma 2.9.** Let  $C(t)$  be as in Definition 1.4. Define, for  $T \geq 0$ ,  $f(T) = \int_{\mathbb{R}^d \setminus [-T, T]^d} 1/(1 + |t|^{d+1}) dt$ . Define, for  $x \in [0, n^{1/d}]^d$ ,  $D_{\Delta}(x) = \inf_{t \in \mathbb{R}^d \setminus C(x)} |x - t|$ . Define  $D_{\Delta}(x_1, \dots, x_m) = \min_{i=1, \dots, m} D_{\Delta}(x_i)$ . Then, there exists a finite constant  $C_{sup}$  so that, for any  $n$ , for any  $x_1, x_2 \in [0, n^{1/d}]^d$ ,

$$\int_{\mathbb{R}^d} \frac{1}{1 + |x_1 - x|^{d+1}} \frac{1}{1 + |x_2 - x|^{d+1}} \mathbf{1}_{C(x) \neq C(x_1)} \mathbf{1}_{C(x) \neq C(x_2)} dx \leq C_{sup} f(D_{\Delta}(x_1, x_2)) \frac{1}{1 + |x_1 - x_2|^{d+1}}.$$

**Lemma 2.10.** Use the notation  $n_2, \Delta, C(t), f(T)$  and  $D_{\Delta}(x_1, x_2)$  of Definition 1.4 and Lemma 2.9. Then, when  $n_2 = o(n)$ ,

$$\frac{1}{n} \int_{[0, n^{1/d}]^d} dx_1 \int_{[0, n^{1/d}]^d} dx_2 \frac{1}{1 + |x_1 - x_2|^{d+1}} f(D_{\Delta}(x_1, x_2)) \rightarrow_{n \rightarrow \infty} 0.$$

**Lemma 2.11.** Use the notation  $n_2, \Delta$  and  $C_1, \dots, C_{n_2}$  of Definition 1.4. Let, for  $i = 1, \dots, n_2$ ,  $X_1^i, \dots, X_{N_i}^i$  be the  $N_i$  components of  $X$  that are in  $C_i$  (so that the order of their indexes in  $X$  is preserved). Then

- i) For  $i = 1, \dots, n_2$ ,  $N_i$  follows a binomial  $B(n, 1/n_2)$  distribution. For any  $i, j = 1, \dots, n_2; i \neq j$ , conditionally to  $N_i = k_i$ ,  $N_j$  follows a binomial  $B(n - k_i, 1/(n_2 - 1))$  distribution.
- ii) Conditionally to  $N_i = k_i$ ,  $X_1^i, \dots, X_{k_i}^i$  are independent and uniformly distributed on  $C_i$ .
- iii) For  $1 \leq i \neq j \leq n_2$ , conditionally to  $N_i = k_i, N_j = k_j$ , the sets of random variables  $(X_1^i, \dots, X_{k_i}^i)$  and  $(X_1^j, \dots, X_{k_j}^j)$  are independent, and their components are independent and uniformly distributed on  $C_i$  and  $C_j$  respectively.

Consider  $n_2$  real-valued functions  $f_1, \dots, f_{n_2}$  of  $X$  that can be written  $f_i(X) = \bar{f}(N_i, X_1^i, \dots, X_{N_i}^i)$ , and so that, for any  $t \in \mathbb{R}^d$ ,  $x_1, \dots, x_N \in \mathbb{R}^d$ ,  $\bar{f}(N, x_1 + t, \dots, x_N + t) = \bar{f}(N, x_1, \dots, x_N)$ . Then

- iv) The variables  $f_1(X), \dots, f_{n_2}(X)$  have the same distribution. The couples  $(f_i(X), f_j(X))$ , for  $1 \leq i \neq j \leq n_2$ , have the same distribution.

**Lemma 2.12.** Use the notation of Lemma 2.11, and consider  $n_2$  functions  $f_1, \dots, f_{n_2}$  that satisfy the conditions of Lemma 2.11. Assume that there exist fixed even natural numbers  $q, l$  and a finite constant  $C_{sup}$  (independent of  $n$  and  $X$ ) so that  $\mathbb{E}(f_i^2(X) | N_i = k) \leq C_{sup}(1 + k^q + k^{q+l}/\Delta^l)$ . Then, if  $\Delta \rightarrow_{n \rightarrow \infty} +\infty$  and  $\Delta = O(n^{1/(2q+5)})$ ,

$$\text{var} \left( \frac{1}{n_2} \sum_{i=1}^{n_2} f_i(X) \right) \rightarrow_{n \rightarrow \infty} 0.$$

**Lemma 2.13.** Let  $N$  follows the binomial distribution  $B(n, 1/n_2)$ , with  $n/n_2 = \Delta \rightarrow_{n \rightarrow \infty} +\infty$ . Then, for any  $k \in \mathbb{N}$ , there exists a finite constant  $C_{sup}$ , independent of  $n$ , so that

$$\mathbb{E}(N^k) \leq C_{sup} \Delta^k.$$

**Lemma 2.14.** Let  $n_2$ ,  $\Delta$  and  $C_1, \dots, C_{n_2}$  be as in Definition 1.4. Assume that  $\Delta$  is lower-bounded, as a function of  $n$ . Then, there exists a finite constant  $C_{sup}$  so that for any  $n$ ,  $i \in \{1, \dots, n_2\}$ ,

$$\sum_{j=1}^{n_2} \frac{1}{1 + d(C_i, C_j)^{d+1}} \leq C_{sup}.$$

**Lemma 2.15.** Let  $A$  be a real  $m_1 \times m_2$  matrix and  $b$  be a  $m_2$ -dimensional real column vector. Then

$$||Ab||^2 \leq m_1 m_2 \left( \max_{i,j} A_{i,j}^2 \right) ||b||^2.$$

### 3 Proof of the technical results

*Proof of Lemma 2.1.* We use a version of the Sobolev embedding theorem on the space  $\Theta$ , equipped with the Lebesgue measure (Theorem 4.12, Part I, Case A in Adams and Fournier (2003)). This result implies that, for any fixed  $X, y$ , there exists a constant  $C_{sup}$  (depending only of  $\Theta$ ) so that

$$\sup_{\theta \in \Theta} |f_\theta(X, y)| \leq C_{sup} \sum_{i_1 + \dots + i_p \leq p} \int_{\Theta} \left| \frac{\partial^{i_1}}{\partial \theta_{i_1}} \dots \frac{\partial^{i_p}}{\partial \theta_{i_p}} f_\theta(X, y) \right| d\theta.$$

By applying the mean value w.r.t  $X$  and  $y$  to this last inequality, and by using Fubini theorem, we prove the lemma.  $\square$

*Proof of Lemma 2.2.* Let  $D_a = \{c \in \mathbb{R}^d; |a - c| \leq |b - c|\}$  and  $D_b = \{c \in \mathbb{R}^d; |b - c| < |a - c|\}$ . Note that, for  $c \in D_a$ ,  $|b - c| \geq |a - b|/2$  and that, for  $c \in D_b$ ,  $|a - c| \geq |a - b|/2$ . Then,

$$\begin{aligned} \int_{\mathbb{R}^d} \frac{1}{1 + |a - c|^{d+1}} \frac{1}{1 + |b - c|^{d+1}} dc &\leq \int_{D_a} \frac{1}{1 + |a - c|^{d+1}} \frac{1}{1 + \left(\frac{|a-b|}{2}\right)^{d+1}} dc \\ &\quad + \int_{D_b} \frac{1}{1 + \left(\frac{|a-b|}{2}\right)^{d+1}} \frac{1}{1 + |b - c|^{d+1}} dc \\ &\leq \frac{1}{1 + |a - b|^{d+1}} 2^{d+1} 2 \int_{\mathbb{R}^d} \frac{1}{1 + |c|^{d+1}} dc. \end{aligned}$$

$\square$

The proof of Lemma 2.3 uses the two following lemmas.

**Lemma 3.1.** There exists a finite constant  $C_{sup}$  so that, for any  $a, b, c \in \mathbb{R}^d$ ,

$$\frac{1}{1 + |a - c|^{d+1}} \frac{1}{1 + |b - c|^{d+1}} \leq C_{sup} \frac{1}{1 + |a - b|^{d+1}}.$$

*Proof of Lemma 3.1.* We have either  $|a - c| \geq |a - b|/2$  or  $|b - c| \geq |a - b|/2$ . The two cases are symmetric. Assume for example  $|a - c| \geq |a - b|/2$ . Then,

$$\frac{1}{1 + |a - c|^{d+1}} \frac{1}{1 + |b - c|^{d+1}} \leq \frac{1}{1 + \left(\frac{|a-b|}{2}\right)^{d+1}} \leq 2^{d+1} \frac{1}{1 + |a - b|^{d+1}}.$$

$\square$

**Lemma 3.2.** There exists a finite constant  $C_{sup}$  so that, for any  $a, b, c \in \mathbb{R}^d$ ,

$$\int_{\mathbb{R}^d} \left( \frac{1}{1 + |a - t|^{d+1}} \right)^2 \frac{1}{1 + |b - t|^{d+1}} \frac{1}{1 + |c - t|^{d+1}} dt \leq C_{sup} \frac{1}{1 + |a - b|^{d+1}} \frac{1}{1 + |a - c|^{d+1}}.$$

*Proof of Lemma 3.2.*

$$\begin{aligned}
& \int_{\mathbb{R}^d} \left( \frac{1}{1 + |a - t|^{d+1}} \right)^2 \frac{1}{1 + |b - t|^{d+1}} \frac{1}{1 + |c - t|^{d+1}} dt \\
& \leq C_{sup} \int_{\mathbb{R}^d} \frac{1}{1 + |a - t|^{d+1}} \frac{1}{1 + |a - b|^{d+1}} \frac{1}{1 + |c - t|^{d+1}} dt \quad (\text{Lemma 3.1}) \\
& \leq C_{sup} \frac{1}{1 + |a - b|^{d+1}} \frac{1}{1 + |a - c|^{d+1}} \quad (\text{Lemma 2.2}).
\end{aligned}$$

□

*Proof of Lemma 2.3.* We can consider without loss of generality that the matrices  $A_1, \dots, A_k$  have non-negative coefficients, since this only increases the quantity  $\mathbb{E}_X(|A_1 \dots A_k|^2)$  to upper bound. Then, note that it is enough to prove the lemma for  $s_n = n$ . Indeed, note first that for  $s_n \neq n$ , it is sufficient to prove the lemma under the following condition (since  $n/s_n$  is lower and upper bounded).

$$(A_l)_{i,j} \leq \frac{1}{1 + \left( \frac{\bar{X}_i - \bar{X}_j}{(n/s_n)^{1/d}} \right)^{d+1}}. \quad (1)$$

Now, if  $s_n \neq n$  observation points are independent and uniformly distributed on  $[0, n^{1/d}]^d$  and the condition on the matrices is (1), then the value of  $\mathbb{E}_X(|A_1 \dots A_k|^2)$  can be seen as an element of the sequence of the same expression, but with  $n$  independent points uniformly distributed on  $[0, n^{1/d}]^d$ , and where the matrices satisfy the condition given in the lemma. This latter sequence is bounded, so also the set of all the values of  $\mathbb{E}_X(|A_1 \dots A_k|^2)$ , for all the values of  $s_n$ , is bounded.

We can hence consider  $s_n = n$  in the proof of the lemma and write, for simplicity,  $\bar{X}_1, \dots, \bar{X}_n$  as the  $n$  standard observation points  $X_1, \dots, X_n$ . Let us first show the lemma for  $k = 1$ .

$$\begin{aligned}
\mathbb{E}_X(|A_1|^2) & \leq \mathbb{E}_X \left[ \frac{1}{n} \sum_{i,j=1}^n \frac{1}{1 + |X_i - X_j|^{d+1}} \right] \\
& \leq \frac{1}{n} \left( n + n^2 \frac{1}{n^2} \int_{[0, n^{1/d}]^d} dx_1 \int_{[0, n^{1/d}]^d} dx_2 \frac{1}{1 + |x_1 - x_2|^{d+1}} \right) \\
& \leq \frac{1}{n} \left( n + \int_{[0, n^{1/d}]^d} dx_1 \int_{\mathbb{R}^d} dx_2 \frac{1}{1 + |x_2|^{d+1}} \right) \\
& \leq C_{sup}.
\end{aligned}$$

The proof of the lemma for  $k = 2$  is similar to but simpler than the proof for  $k \geq 3$ , that we now do. Thus, for the rest of the proof, we consider  $k \geq 3$ . We have

$$\begin{aligned}
& \mathbb{E}_X(|A_1 \dots A_k|^2) \\
& = \frac{1}{n} \mathbb{E}_X \sum_{i,j=1}^n \left[ \sum_{a_1=1}^n (A_1)_{i,a_1} (A_2 \dots A_k)_{a_1,j} \right]^2 \\
& = \frac{1}{n} \mathbb{E}_X \sum_{i,j=1}^n \left[ \sum_{a_1,a_2=1}^n (A_1)_{i,a_1} (A_2)_{a_1,a_2} (A_3 \dots A_k)_{a_2,j} \right]^2 \\
& = \frac{1}{n} \mathbb{E}_X \sum_{i,j=1}^n \left[ \sum_{a_1,a_2,\dots,a_{k-1}=1}^n (A_1)_{i,a_1} (A_2)_{a_1,a_2} \dots (A_k)_{a_{k-1},j} \right]^2 \\
& = \frac{1}{n} \mathbb{E}_X \sum_{i,j=1}^n \sum_{a_1,a_2,\dots,a_{k-1}=1}^n \sum_{b_1,b_2,\dots,b_{k-1}=1}^n (A_1)_{i,a_1} (A_2)_{a_1,a_2} \dots (A_k)_{a_{k-1},j} (A_1)_{i,b_1} (A_2)_{b_1,b_2} \dots (A_k)_{b_{k-1},j}.
\end{aligned} \quad (2)$$

Define

$$S_{j,a_{k-2},b_{k-2}} := \sum_{a_{k-1},b_{k-1}=1}^n (A_{k-1})_{a_{k-2},a_{k-1}} (A_k)_{a_{k-1},j} (A_{k-1})_{b_{k-2},b_{k-1}} (A_k)_{b_{k-1},j}. \quad (3)$$

Then we have

$$\begin{aligned} \mathbb{E}_X (|A_1 \dots A_k|^2) &= \\ \frac{1}{n} \mathbb{E}_X \sum_{i,j=1}^n \sum_{a_1,a_2,\dots,a_{k-2}=1}^n \sum_{b_1,b_2,\dots,b_{k-2}=1}^n \\ (A_1)_{i,a_1} (A_2)_{a_1,a_2} \dots (A_{k-2})_{a_{k-3},a_{k-2}} (A_1)_{i,b_1} (A_2)_{b_1,b_2} \dots (A_{k-2})_{b_{k-3},b_{k-2}} S_{j,a_{k-2},b_{k-2}}. \end{aligned}$$

We write  $X_{i,j,a_1,\dots,a_{k-2},b_1,\dots,b_{k-2}}$  as a shorthand for the  $(2k-2)$ -tuple of random variables

$$(X_i, X_j, X_{a_1}, \dots, X_{a_{k-2}}, X_{b_1}, \dots, X_{b_{k-2}}).$$

We now show that, to prove the lemma by induction on  $k$ , it is sufficient to show that there exists a finite constant  $C_{sup}$  so that, for any values of the indexes  $i, j, a_1, \dots, a_{k-2}, b_1, \dots, b_{k-2}$ , and for any realization of the corresponding variable  $X_{i,j,a_1,\dots,a_{k-2},b_1,\dots,b_{k-2}}$ ,

$$\mathbb{E} (|S_{j,a_{k-2},b_{k-2}}| | X_{i,j,a_1,\dots,a_{k-2},b_1,\dots,b_{k-2}}) \leq C_{sup} \frac{1}{1 + |X_{a_{k-2}} - X_j|^{d+1}} \frac{1}{1 + |X_{b_{k-2}} - X_j|^{d+1}}. \quad (4)$$

Indeed, we have

$$\begin{aligned} \mathbb{E}_X (|A_1 \dots A_k|^2) &= \\ \frac{1}{n} \mathbb{E}_X \sum_{i,j=1}^n \sum_{a_1,a_2,\dots,a_{k-2}=1}^n \sum_{b_1,b_2,\dots,b_{k-2}=1}^n \\ (A_1)_{i,a_1} (A_2)_{a_1,a_2} \dots (A_{k-2})_{a_{k-3},a_{k-2}} (A_1)_{i,b_1} (A_2)_{b_1,b_2} \dots (A_{k-2})_{b_{k-3},b_{k-2}} S_{j,a_{k-2},b_{k-2}} \\ &= \frac{1}{n} \sum_{i,j=1}^n \sum_{a_1,a_2,\dots,a_{k-2}=1}^n \sum_{b_1,b_2,\dots,b_{k-2}=1}^n \\ \mathbb{E}_{X_{i,j,a_1,\dots,a_{k-2},b_1,\dots,b_{k-2}}} [(A_1)_{i,a_1} (A_2)_{a_1,a_2} \dots (A_{k-2})_{a_{k-3},a_{k-2}} (A_1)_{i,b_1} (A_2)_{b_1,b_2} \dots (A_{k-2})_{b_{k-3},b_{k-2}}] \\ &\quad \mathbb{E} (S_{j,a_{k-2},b_{k-2}} | X_{i,j,a_1,\dots,a_{k-2},b_1,\dots,b_{k-2}}). \end{aligned}$$

With the consideration that  $A_1, \dots, A_k$  have non-negative coefficients we have, under (4),

$$\begin{aligned} \mathbb{E}_X (|A_1 \dots A_k|^2) &\leq C_{sup} \frac{1}{n} \sum_{i,j=1}^n \sum_{a_1,a_2,\dots,a_{k-2}=1}^n \sum_{b_1,b_2,\dots,b_{k-2}=1}^n \\ \mathbb{E}_{X_{i,j,a_1,\dots,a_{k-2},b_1,\dots,b_{k-2}}} [(A_1)_{i,a_1} (A_2)_{a_1,a_2} \dots (A_{k-2})_{a_{k-3},a_{k-2}} (A_1)_{i,b_1} (A_2)_{b_1,b_2} \dots (A_{k-2})_{b_{k-3},b_{k-2}}] \\ &\quad \frac{1}{1 + |X_{a_{k-2}} - X_j|^{d+1}} \frac{1}{1 + |X_{b_{k-2}} - X_j|^{d+1}}. \end{aligned}$$

By defining  $\tilde{A}_{k-1}$  by  $(\tilde{A}_{k-1})_{c,d} = 1/(1 + |X_c - X_d|^{d+1})$ , we obtain

$$\begin{aligned} \mathbb{E}_X (|A_1 \dots A_k|^2) &\leq \frac{C_{sup}}{n} \mathbb{E}_X \sum_{i,j=1}^n \sum_{a_1,a_2,\dots,a_{k-2}=1}^n \sum_{b_1,b_2,\dots,b_{k-2}=1}^n \\ (A_1)_{i,a_1} (A_2)_{a_1,a_2} \dots (\tilde{A}_{k-1})_{a_{k-2},j} (A_1)_{i,b_1} (A_2)_{b_1,b_2} \dots (\tilde{A}_{k-1})_{b_{k-2},j} \\ &= C_{sup} \mathbb{E}_X (|A_1 A_2 \dots \tilde{A}_{k-1}|^2) \quad \text{from (2)}. \end{aligned}$$

Thus, if (4) holds, we can prove the lemma by induction on  $k$ . Let us now prove (4). This is done by writing

$$\begin{aligned} S_{j,a_{k-2},b_{k-2}} &= \sum_{\substack{n \\ a_{k-1},b_{k-1}=1}} (A_{k-1})_{a_{k-2},a_{k-1}} (A_k)_{a_{k-1},j} (A_{k-1})_{b_{k-2},b_{k-1}} (A_k)_{b_{k-1},j} \\ &= \sum_{c=1}^4 \sum_{(a_{k-1},b_{k-1}) \in I_c} (A_{k-1})_{a_{k-2},a_{k-1}} (A_k)_{a_{k-1},j} (A_{k-1})_{b_{k-2},b_{k-1}} (A_k)_{b_{k-1},j}, \end{aligned}$$

where the sets of indices  $I_1, \dots, I_4$  are defined below and form a partition of  $\{1, \dots, n\}^2$ . It is then sufficient to show that for  $c = 1, \dots, 4$ , there exists a finite constant  $C_{sup}$  so that for any  $(a, b) \in I_c$ ,

$$\begin{aligned} &|I_c| \mathbb{E} \left\{ \frac{1}{1 + |X_{a_{k-2}} - X_a|^{d+1}} \frac{1}{1 + |X_a - X_j|^{d+1}} \frac{1}{1 + |X_{b_{k-2}} - X_b|^{d+1}} \frac{1}{1 + |X_b - X_j|^{d+1}} \right. \\ &\quad \left. X_{i,j,a_1,\dots,a_{k-2},b_1,\dots,b_{k-2}} \right\} \\ &\leq C_{sup} \frac{1}{1 + |X_{a_{k-2}} - X_j|^{d+1}} \frac{1}{1 + |X_{b_{k-2}} - X_j|^{d+1}}. \end{aligned} \quad (5)$$

We define the set  $I_1$  as the set of the  $a, b \in \{1, \dots, n\}$  that are different, and that do not belong to the set  $\{i, j, a_1, \dots, a_{k-2}, b_1, \dots, b_{k-2}\}$ . For  $I_1$ , the cardinality in (5) is less than  $n^2$  and the conditional mean values in (5) are equal to

$$\begin{aligned} &\frac{1}{n^2} \left( \int_{[0,n^{1/d}]^d} \frac{1}{1 + |X_{a_{k-2}} - x_a|^{d+1}} \frac{1}{1 + |x_a - X_j|^{d+1}} dx_a \right) \\ &\left( \int_{[0,n^{1/d}]^d} \frac{1}{1 + |X_{b_{k-2}} - x_b|^{d+1}} \frac{1}{1 + |x_b - X_j|^{d+1}} dx_b \right), \end{aligned}$$

so that (5) holds because of Lemma 2.2. We define the set  $I_2$  as the set of the  $a, b \in \{1, \dots, n\}$  that are equal, and that do not belong to the set  $\{i, j, a_1, \dots, a_{k-2}, b_1, \dots, b_{k-2}\}$ . For  $I_2$ , the cardinality in (5) is less than  $n$  and the conditional mean values in (5) are equal to

$$\frac{1}{n} \int_{[0,n^{1/d}]^d} \frac{1}{1 + |X_{a_{k-2}} - x_a|^{d+1}} \frac{1}{1 + |x_a - X_j|^{d+1}} \frac{1}{1 + |X_{b_{k-2}} - x_a|^{d+1}} \frac{1}{1 + |x_a - X_j|^{d+1}} dx_a,$$

so that (5) holds because of Lemma 3.2. We define the set  $I_3$  as the set of the  $a, b \in \{1, \dots, n\}$  that are so that one of them is in the set  $\{i, j, a_1, \dots, a_{k-2}, b_1, \dots, b_{k-2}\}$  and the other one is not in the set  $\{i, j, a_1, \dots, a_{k-2}, b_1, \dots, b_{k-2}\}$ . For  $I_3$ , the cardinality in (5) is less than  $C_{sup}n$ . For the conditional mean values in (5), by symmetry, we can assume  $a \in \{i, j, a_1, \dots, a_{k-2}, b_1, \dots, b_{k-2}\}$ . Then, the conditional mean values in (5) are equal to

$$\begin{aligned} &\frac{1}{n} \int_{[0,n^{1/d}]^d} \frac{1}{1 + |X_{a_{k-2}} - X_a|^{d+1}} \frac{1}{1 + |X_a - X_j|^{d+1}} \frac{1}{1 + |X_{b_{k-2}} - x_b|^{d+1}} \frac{1}{1 + |x_b - X_j|^{d+1}} dx_b \\ &\leq C_{sup} \frac{1}{n} \frac{1}{1 + |X_{a_{k-2}} - X_j|^{d+1}} \int_{[0,n^{1/d}]^d} \frac{1}{1 + |X_{b_{k-2}} - x_b|^{d+1}} \frac{1}{1 + |x_b - X_j|^{d+1}} dx_b \quad (\text{Lemma 3.1}) \\ &\leq C_{sup} \frac{1}{n} \frac{1}{1 + |X_{a_{k-2}} - X_j|^{d+1}} \frac{1}{1 + |X_{b_{k-2}} - X_j|^{d+1}} \quad (\text{Lemma 2.2}). \end{aligned}$$

Finally, we define the set  $I_4$  as the set of the  $a, b \in \{1, \dots, n\}$  that both belong to the set  $\{i, j, a_1, \dots, a_{k-2}, b_1, \dots, b_{k-2}\}$ . For  $I_4$ , the cardinality in (5) is bounded (w.r.t  $n$ ) and the conditional mean values in (5) are equal to

$$\frac{1}{1 + |X_{a_{k-2}} - X_a|^{d+1}} \frac{1}{1 + |X_a - X_j|^{d+1}} \frac{1}{1 + |X_{b_{k-2}} - X_b|^{d+1}} \frac{1}{1 + |X_b - X_j|^{d+1}},$$

so that (5) holds because of Lemma 3.1. Thus, (4) is proved, which completes the proof of the lemma.  $\square$

*Proof of Lemma 2.4.* We show the lemma for  $R_\theta^{-1}$ ,  $\text{diag}(R_\theta^{-1})$  and  $\text{diag}(R_\theta^{-1})^{-1}$ , the proof for  $R_{1,\theta}^{-1}$ ,  $\text{diag}(R_{1,\theta}^{-1})$  and  $\text{diag}(R_{1,\theta}^{-1})^{-1}$  being similar. The matrix  $R_\theta$  is the sum of a symmetric non-negative matrix and of  $\delta_\theta I_n$ . Thus, the eigenvalues of its inverse are smaller than  $1/C_{inf}$  from Condition 1.3. Then, from Lemma D.6 in Bachoc (2014), the eigenvalues of  $\text{diag}(R_\theta^{-1})$  are also smaller than  $1/C_{inf}$ . Finally, from Proposition 0.1 in the supplementary material of Bachoc (2013),  $(\text{diag}(R_\theta^{-1})^{-1})_{i,i} = K_\theta(0) + \delta_\theta - r_{1,\theta}^t R_{1,\theta}^{-1} r_{1,\theta} \leq C_{sup}$ , from Condition 1.3.  $\square$

*Proof of Lemma 2.5.* Same as for Lemma 2.4.  $\square$

*Proof of Lemma 2.6.* Same as for Lemma 2.4.  $\square$

*Proof of Lemma 2.7.* We have, for any  $\theta \in \Theta$ ,

$$\begin{aligned}
\mathbb{E}_X |B_{1,\theta} A_{1,\theta} B_{2,\theta} \dots B_{k,\theta} A_{k,\theta} B_{k+1,\theta}|^2 &\leq C_{sup} \mathbb{E}_X |A_{1,\theta} B_{2,\theta} \dots B_{k,\theta} A_{k,\theta}|^2 \\
&= C_{sup} \mathbb{E}_X \frac{1}{n} \text{Tr} (A_{1,\theta} B_{2,\theta} \dots B_{k,\theta} A_{k,\theta} A_{k,\theta} B_{k,\theta} \dots B_{2,\theta} A_{1,\theta}) \\
&= C_{sup} \mathbb{E}_X \frac{1}{n} \text{Tr} (A_{1,\theta}^2 B_{2,\theta} \dots B_{k,\theta} A_{k,\theta}^2 B_{k,\theta} \dots B_{2,\theta}) \\
(\text{Cauchy Schwarz:}) &\leq \sqrt{\mathbb{E}_X |A_{1,\theta}^2 B_{2,\theta} \dots B_{k,\theta}|^2} \sqrt{\mathbb{E}_X |A_{k,\theta}^2 B_{k,\theta} \dots B_{2,\theta}|^2} \\
&\leq C_{sup} \sqrt{\mathbb{E}_X |A_{1,\theta}^2 B_{2,\theta} \dots A_{k-1,\theta}|^2} \sqrt{\mathbb{E}_X |A_{k,\theta}^2 B_{k,\theta} \dots A_{2,\theta}|^2}.
\end{aligned} \tag{6}$$

Both of the square roots in (6) are applied to a term of the form

$$\mathbb{E}_X |B'_{1,\theta} A'_{1,\theta} B'_{2,\theta} \dots B'_{k-1,\theta} A'_{k-1,\theta} B'_{k,\theta}|^2,$$

where the sequences of random matrices  $B'_{1,\theta}, A'_{1,\theta}, B'_{2,\theta}, \dots, B'_{k-1,\theta}, A'_{k-1,\theta}, B'_{k,\theta}$  satisfy the conditions of the lemma. Thus, we have shown that we can reduce the problem involving  $k$  matrices  $A_{1,\theta}, \dots, A_{k,\theta}$  to a similar problem involving  $k-1$  matrices  $A_{1,\theta}, \dots, A_{k-1,\theta}$ . On the other hand, the result is true by assumption for  $k=1$ . Thus, we have proved the lemma by induction on  $k$ .  $\square$

*Proof of Lemma 2.8.* Let us write  $F_{i,j}$  and  $C_{i,j}$  as shorthands for  $1/(1 + |X_i - X_j|^{d+1})$  and  $\mathbf{1}_{C(X_i) \neq C(X_j)}$ . Let us also write  $i_1 \neq i_2 \neq \dots \neq i_k$  when  $k$  numbers  $i_1, \dots, i_k$  are two-by-two distinct. Then we have, from Condition 1.3,

$$\begin{aligned}
& \mathbb{E} \left( \left| (R_{1,\theta} - \tilde{R}_{1,\theta})^2 \right|^2 \right) \\
&= \frac{1}{n} \sum_{i,j,k,l=2}^n \mathbb{E} \left( (R_{1,\theta} - \tilde{R}_{1,\theta})_{i,k} (R_{1,\theta} - \tilde{R}_{1,\theta})_{k,j} (R_{1,\theta} - \tilde{R}_{1,\theta})_{i,l} (R_{1,\theta} - \tilde{R}_{1,\theta})_{l,j} \right) \\
&\leq C_{sup} \frac{1}{n} \sum_{i,j,k,l=2}^n \mathbb{E} (C_{i,k} C_{k,j} C_{i,l} C_{l,j} F_{i,k} F_{k,j} F_{i,l} F_{l,j}) \\
&= C_{sup} \frac{1}{n} \sum_{i,j=2}^n \sum_{\substack{k=2,\dots,n \\ k \notin \{i,j\}}} \mathbb{E} (C_{i,k}^2 C_{k,j}^2 F_{i,k}^2 F_{k,j}^2) \\
&\quad + C_{sup} \frac{1}{n} \sum_{i,j=2}^n \sum_{\substack{k,l=2,\dots,n \\ k \neq l, k,l \notin \{i,j\}}} \mathbb{E} (C_{i,k} C_{k,j} C_{i,l} C_{l,j} F_{i,k} F_{k,j} F_{i,l} F_{l,j}).
\end{aligned}$$

Hence, by distinguishing  $i = j$  from  $i \neq j$  in each of the two double sums in the above display, and by noting that two of the four corresponding cases are symmetric, we obtain

$$\begin{aligned}
\mathbb{E} \left( \left| (R_{1,\theta} - \tilde{R}_{1,\theta})^2 \right|^2 \right) &\leq C_{sup} \frac{1}{n} \sum_{\substack{i,k=2,\dots,n \\ i \neq k}} \mathbb{E} (C_{i,k} F_{i,k}) + C_{sup} \frac{1}{n} \sum_{\substack{i,j,k=2,\dots,n \\ i \neq j \neq k}} \mathbb{E} (C_{i,k} C_{k,j} F_{i,k} F_{k,j}) \\
&\quad + C_{sup} \frac{1}{n} \sum_{\substack{i,j,k,l=2,\dots,n \\ i \neq j \neq k \neq l}} \mathbb{E} (C_{i,k} C_{k,j} C_{i,l} C_{l,j} F_{i,k} F_{k,j} F_{i,l} F_{l,j}) \\
&\leq C_{sup} \frac{1}{n} n^2 \mathbb{E} (C_{1,2} F_{1,2}) + C_{sup} \frac{1}{n} n^3 \mathbb{E} (C_{1,3} C_{3,2} F_{1,3} F_{3,2}) \\
&\quad + C_{sup} \frac{1}{n} n^4 \mathbb{E} (C_{1,3} C_{3,2} C_{1,4} C_{4,2} F_{1,3} F_{3,2} F_{1,4} F_{4,2}) \quad (\text{by symmetry}).
\end{aligned} \tag{7}$$

Let us call  $T_1$ ,  $T_2$  and  $T_3$  the three terms in (7). For the term  $T_1$ ,

$$\begin{aligned}
T_1 &= \frac{1}{n} \int_{[0, n^{1/d}]^d} dx_1 \int_{[0, n^{1/d}]^d} dx_2 \frac{1}{1 + |x_1 - x_2|^{d+1}} \mathbf{1}_{C(x_1) \neq C(x_2)} \\
&\leq \frac{1}{n} \int_{[0, n^{1/d}]^d} dx_1 f(D_\Delta(x_1)) \quad (\text{notation of Lemma 2.9}).
\end{aligned}$$

Now, for any  $\epsilon > 0$ , there is a finite  $T$  so that  $f(T) \leq \epsilon$ , and by defining  $E_n = \{x \in [0, n^{1/d}]^d; D_\Delta(x) \leq T\}$ , we have  $|E_n| = o(n)$ , as can be seen easily, and

$$\frac{1}{n} \int_{[0, n^{1/d}]^d} f(D_\Delta(x_1)) dx_1 \leq f(0) \frac{|E_n|}{n} + \epsilon,$$

to that  $T_1 \rightarrow_{n \rightarrow \infty} 0$ . For the term  $T_2$ ,

$$\begin{aligned}
T_2 &= \frac{1}{n} \int_{[0, n^{1/d}]^d} dx_1 \int_{[0, n^{1/d}]^d} dx_2 \int_{[0, n^{1/d}]^d} dx_3 \frac{1}{1 + |x_1 - x_3|^{d+1}} \frac{1}{1 + |x_2 - x_3|^{d+1}} \mathbf{1}_{C(x_1) \neq C(x_3)} \mathbf{1}_{C(x_2) \neq C(x_3)} \\
&\leq \frac{1}{n} \int_{[0, n^{1/d}]^d} dx_1 \int_{[0, n^{1/d}]^d} dx_2 \frac{1}{1 + |x_1 - x_2|^{d+1}} f(D_\Delta(x_1, x_2)) \quad (\text{Lemma 2.9}) \\
&\rightarrow_{n \rightarrow \infty} 0 \quad (\text{Lemma 2.10.})
\end{aligned}$$

For the term  $T_3$ ,

$T_3 =$

$$\begin{aligned} & \frac{1}{n} \int_{[0, n^{1/d}]^d} dx_1 \int_{[0, n^{1/d}]^d} dx_2 \int_{[0, n^{1/d}]^d} dx_3 \int_{[0, n^{1/d}]^d} dx_4 \\ & \frac{1}{1 + |x_1 - x_3|^{d+1}} \frac{1}{1 + |x_2 - x_3|^{d+1}} \frac{1}{1 + |x_1 - x_4|^{d+1}} \frac{1}{1 + |x_2 - x_4|^{d+1}} \\ & \mathbf{1}_{C(x_1) \neq C(x_3)} \mathbf{1}_{C(x_2) \neq C(x_3)} \mathbf{1}_{C(x_1) \neq C(x_4)} \mathbf{1}_{C(x_2) \neq C(x_4)} \\ & \leq C_{sup} \frac{1}{n} \int_{[0, n^{1/d}]^d} dx_1 \int_{[0, n^{1/d}]^d} dx_2 \left( \frac{1}{1 + |x_1 - x_2|^{d+1}} \right)^2 f^2(D_\Delta(x_1, x_2)) \quad (\text{from Lemma 2.9.}) \end{aligned}$$

Now, because  $f(t) \rightarrow_{t \rightarrow +\infty} 0$ , is continuous and positive, there exists a finite  $C_{sup}$  so that  $f^2 \leq C_{sup} f$ . Thus, we can conclude from Lemma 2.10.  $\square$

*Proof of Lemma 2.9.* Let  $T = D_\Delta(x_1, x_2)$ . Let  $B_{x_1} = \{x \in \mathbb{R}^d, |x - x_1| < T\}$ ,  $B_{x_2} = \{x \in \mathbb{R}^d, |x - x_2| < T\}$ ,  $A_{x_1} = \{x \in \mathbb{R}^d; |x - x_1| \leq |x - x_2|\}$  and  $A_{x_2} = \{x \in \mathbb{R}^d; |x - x_2| < |x - x_1|\}$ . Observe that  $C(x) \neq C(x_1)$  implies  $x \notin B_{x_1}$ , that  $x \in A_{x_1}$  implies  $|x - x_2| \geq |x_1 - x_2|/2$  and that we have the symmetric results when interchanging the roles of  $x_1$  and  $x_2$ . Then, we obtain

$$\begin{aligned} & \int_{\mathbb{R}^d} \frac{1}{1 + |x - x_1|^{d+1}} \frac{1}{1 + |x - x_2|^{d+1}} \mathbf{1}_{C(x) \neq C(x_1)} \mathbf{1}_{C(x) \neq C(x_2)} dx \\ & \leq \int_{A_{x_1} \setminus B_{x_1}} \frac{1}{1 + |x - x_1|^{d+1}} \frac{1}{1 + \left(\frac{|x_1 - x_2|}{2}\right)^{d+1}} dx + \int_{A_{x_2} \setminus B_{x_2}} \frac{1}{1 + \left(\frac{|x_1 - x_2|}{2}\right)^{d+1}} \frac{1}{1 + |x - x_2|^{d+1}} dx \\ & \leq 2^{d+1} \frac{1}{1 + |x_1 - x_2|^{d+1}} 2f(T). \end{aligned}$$

$\square$

*Proof of Lemma 2.10.* Let  $\epsilon > 0$  and let  $T$  be a constant so that  $f(T) \leq \epsilon$ . Let  $E_n(T) = \{x \in [0, n^{1/d}]^d; D_\Delta(x) \leq T\}$ . Then,

$$\begin{aligned} \frac{1}{n} \int_{E_n(T)} dx_1 \int_{[0, n^{1/d}]^d} dx_2 \frac{1}{1 + |x_1 - x_2|^{d+1}} f(D_\Delta(x_1, x_2)) & \leq \frac{|E_n(T)|}{n} f(0) \int_{\mathbb{R}^d} \frac{1}{1 + |t|^{d+1}} dt \\ & \xrightarrow{n \rightarrow \infty} 0. \end{aligned}$$

Also,

$$\begin{aligned} & \frac{1}{n} \int_{[0, n^{1/d}]^d \setminus E_n(T)} dx_1 \int_{[0, n^{1/d}]^d} dx_2 \frac{1}{1 + |x_1 - x_2|^{d+1}} f(D_\Delta(x_1, x_2)) \\ & \leq \frac{1}{n} \int_{[0, n^{1/d}]^d \setminus E_n(T)} dx_1 \int_{E_n(T)} dx_2 \frac{1}{1 + |x_1 - x_2|^{d+1}} f(0) \\ & \quad + \frac{1}{n} \int_{[0, n^{1/d}]^d \setminus E_n(T)} dx_1 \int_{[0, n^{1/d}]^d \setminus E_n(T)} dx_2 \frac{1}{1 + |x_1 - x_2|^{d+1}} \epsilon \\ & \quad (\text{by definition of } D_\Delta(x_1, x_2) \text{ and } E_n(\cdot)) \\ & \leq \frac{|E_n(T)|}{n} f(0) \int_{\mathbb{R}^d} \frac{1}{1 + |t|^{d+1}} dt + \epsilon \int_{\mathbb{R}^d} \frac{1}{1 + |t|^{d+1}} dt \quad (\text{by Fubini theorem}) \\ & = o(1) f(0) \int_{\mathbb{R}^d} \frac{1}{1 + |t|^{d+1}} dt + \epsilon \int_{\mathbb{R}^d} \frac{1}{1 + |t|^{d+1}} dt, \end{aligned}$$

which finishes the proof.  $\square$

*Proof of Lemma 2.11.* Because  $X_1, \dots, X_n$  are independent and uniformly distributed on  $[0, n^{1/d}]^d$ , and because  $\frac{|C_i|}{n} = \frac{1}{n_2}$ , the first part of i) holds. For the second part of i), we calculate, for  $i \neq j$ ,

$$\begin{aligned} \frac{P(N_i = k_i; N_j = l_j)}{P(N_i = k_i)} &= \frac{\binom{n}{k_i} \binom{n-k_i}{l_j} \left(\frac{1}{n_2}\right)^{k_i} \left(\frac{1}{n_2}\right)^{l_j} \left(\frac{n_2-2}{n_2}\right)^{n-k_i-l_j}}{\binom{n}{k_i} \left(\frac{1}{n_2}\right)^{k_i} \left(\frac{n_2-1}{n_2}\right)^{n-k_i}} \\ &= \binom{n-k_i}{l_j} \left(\frac{1}{n_2-1}\right)^{l_j} \left(\frac{n_2-2}{n_2-1}\right)^{n-k_i-l_j}, \end{aligned}$$

which proves the second part.

For ii), consider  $i$  and a measurable function  $g(X_1^i, \dots, X_{N_i}^i)$ . Let, for a subset  $C$  of  $\{1, \dots, n\}$ ,  $X_C$  be the tuple built by extracting the elements of  $X$  which indexes are in  $C$ . Also, for  $E \subset \mathbb{R}^d$  and for a  $r$ -tuple  $v = (v_1, \dots, v_r) \in (\mathbb{R}^d)^r$ , we write  $v \in E$  when all the components  $v_1, \dots, v_r$  are in  $E$ . Then we have

$$\begin{aligned} &\frac{\mathbb{E}(g(X_1^i, \dots, X_{N_i}^i) \mathbf{1}_{N_i=k_i})}{P(N_i = k_i)} \\ &= \frac{\mathbb{E}\left(\sum_{k_1 < \dots < k_{k_i} \in \{1, \dots, n\}} g(X_{k_1}, \dots, X_{k_{k_i}}) \mathbf{1}_{X_{\{k_1, \dots, k_{k_i}\}} \in C_i} \mathbf{1}_{X_{\{1, \dots, n\} \setminus \{k_1, \dots, k_{k_i}\}} \in [0, n^{1/d}]^d \setminus C_i}\right)}{\binom{n}{k_i} \left(\frac{1}{n_2}\right)^{k_i} \left(\frac{n_2-1}{n_2}\right)^{n-k_i}} \\ &= \frac{1}{\Delta^{k_i}} \int_{C_i^{k_i}} g(x_1, \dots, x_{k_i}) dx_1 \dots dx_{k_i}. \end{aligned}$$

This proves ii). For iii), consider  $i \neq j$  and two measurable functions  $g(X_1^i, \dots, X_{N_i}^i)$  and  $h(X_1^j, \dots, X_{N_j}^j)$ . Then,

$$\begin{aligned} &\frac{\mathbb{E}(g(X_1^i, \dots, X_{N_i}^i) h(X_1^j, \dots, X_{N_j}^j) \mathbf{1}_{N_i=k_i} \mathbf{1}_{N_j=l_j})}{P(N_i = k_i; N_j = l_j)} \\ &= \sum_{k_1 < \dots < k_{k_i} \in \{1, \dots, n\}} \sum_{l_1 < \dots < l_{l_j} \in \{1, \dots, n\} \setminus \{k_1, \dots, k_{k_i}\}} \\ &\frac{\mathbb{E}\left(g(X_{k_1}, \dots, X_{k_{k_i}}) h(X_{l_1}, \dots, X_{l_{l_j}}) \mathbf{1}_{X_{\{k_1, \dots, k_{k_i}\}} \in C_i} \mathbf{1}_{X_{\{l_1, \dots, l_{l_j}\}} \in C_j} \mathbf{1}_{X_{\{1, \dots, n\} \setminus \{k_1, \dots, k_{k_i}, l_1, \dots, l_{l_j}\}} \in [0, n^{1/d}]^d \setminus (C_i \cup C_j)}\right)}{\binom{n}{k_i} \binom{n-k_i}{l_j} \left(\frac{1}{n_2}\right)^{k_i} \left(\frac{1}{n_2}\right)^{l_j} \left(\frac{n_2-2}{n_2}\right)^{n-k_i-l_j}} \\ &= \frac{1}{\Delta^{k_i}} \int_{C_i^{k_i}} g(x_1, \dots, x_{k_i}) dx_1 \dots dx_{k_i} \frac{1}{\Delta^{l_j}} \int_{C_j^{l_j}} h(x_1, \dots, x_{l_j}) dx_1 \dots dx_{l_j}. \end{aligned}$$

This proves iii). Now, iv) is a consequence of i), ii) and iii). □

The proof of Lemma 2.12 uses the following lemma.

**Lemma 3.3.** Consider two functions of  $n$ :  $\tau(n)$  and  $a(n)$ , that we write  $\tau$  and  $a$  for simplicity and so that  $\tau \rightarrow_{n \rightarrow \infty} 0$ ,  $n\tau \rightarrow_{n \rightarrow \infty} +\infty$  and  $a \rightarrow_{n \rightarrow \infty} +\infty$ . Let  $N$  follow the binomial distribution  $B(n, \tau)$ . Then, for any  $k \in \mathbb{N}$ , there exists a finite constant  $C_{sup}$ , independent of  $n$ , so that,

$$\mathbb{E}(N^k \mathbf{1}_{N \geq a n \tau}) \leq C_{sup} \frac{(n\tau)^{k-1}}{a^2}.$$

*Proof of Lemma 3.3.* For  $k = 0$ , we have, using Chebyshev's inequality,

$$P(N \geq an\tau) \leq \frac{n\tau(1-\tau)}{(a-1)^2(n\tau)^2} \leq \frac{2}{a^2n\tau},$$

for  $n$  large enough. Thus, the lemma holds for  $k = 0$ . Now, for  $k > 0$ , using the convention, for  $t \in \mathbb{R}$ ,  $\sum_{i=t}^n (\cdot) = \sum_{i=1, \dots, n; i \geq t} (\cdot)$ ,

$$\begin{aligned} \mathbb{E}(N^{k+1} \mathbf{1}_{N \geq an\tau}) &= \sum_{i=an\tau}^n i^{k+1} \binom{n}{i} \tau^i (1-\tau)^{n-i} \\ &= n\tau \sum_{i=an\tau-1}^{n-1} (i+1)^k \binom{n-1}{i} \tau^i (1-\tau)^{n-1-i}. \end{aligned}$$

We have  $(i+1)^k \leq 2i^k$  for  $i$  large enough. Thus, with  $\tilde{N}$  following a  $B(n-1, \tau)$  distribution, we have

$$\mathbb{E}(N^{k+1} \mathbf{1}_{N \geq an\tau}) \leq n\tau 2 \mathbb{E}(\tilde{N}^k \mathbf{1}_{\tilde{N} \geq \frac{an\tau-1}{(n-1)\tau} (n-1)\tau}).$$

Finally, the sequences  $n' = (n-1)$ ,  $\tau' = \tau$  and  $a' = (an\tau-1)/((n-1)\tau)$  satisfy the conditions of the lemma. Furthermore,  $a' \geq a/2$  for  $n$  large enough. Thus, we prove the lemma by induction on  $k$ .  $\square$

*Proof of Lemma 2.12.* Because of Lemma 2.11, it is enough to show that  $\text{var}(f_1(X)) = o(n_2)$  and  $\text{cov}(f_1(X), f_2(X)) = o(1)$ .

We have,

$$\begin{aligned} \frac{1}{n_2} \text{var}(f_1(X)) &\leq \frac{1}{n_2} \mathbb{E}[\mathbb{E}(f_1^2(X)|N_1)] \\ &\leq C_{sup} \frac{1}{n_2} \mathbb{E}\left(1 + N_1^q + \frac{N_1^{q+l}}{\Delta^l}\right) \\ &\leq C_{sup} \frac{1}{n_2} \Delta^q \quad (\text{Lemma 2.13}) \\ &= C_{sup} \frac{\Delta^{q+1}}{n}, \end{aligned}$$

which goes to 0 by assumption on  $\Delta$ . Now, using Lemma 2.11

$$\begin{aligned} \text{cov}(f_1(X), f_2(X)) &= \mathbb{E}(f_1(X)f_2(X)) - \mathbb{E}(f_1(X))\mathbb{E}(f_2(X)) \\ &= \sum_{k_1=0}^n \sum_{k_2=0}^n \mathbb{E}(f_1(X)|N_1 = k_1) \mathbb{E}(f_2(X)|N_2 = k_2) \{P(N_1 = k_1, N_2 = k_2) - P(N_1 = k_1)P(N_2 = k_2)\}. \end{aligned}$$

Now,

$$|\mathbb{E}(f_i(X)|N_i = k_i)| \leq \sqrt{\mathbb{E}(f_i^2(X)|N_i = k_i)} \leq C_{sup} \sqrt{\left(1 + k_i^q + \frac{k_i^{q+l}}{\Delta^l}\right)} \leq C_{sup} \left(1 + k_i^{\frac{q}{2}} + \frac{k_i^{\frac{q+l}{2}}}{\Delta^{\frac{l}{2}}}\right).$$

Hence,

$$\begin{aligned} \text{cov}(f_1(X), f_2(X)) & \tag{8} \\ &\leq \sum_{k_1=0}^n \left(1 + k_1^{\frac{q}{2}} + \frac{k_1^{\frac{q+l}{2}}}{\Delta^{\frac{l}{2}}}\right) P(N_1 = k_1) \left\{ \sum_{k_2=0}^n \left(1 + k_2^{\frac{q}{2}} + \frac{k_2^{\frac{q+l}{2}}}{\Delta^{\frac{l}{2}}}\right) |P(N_2 = k_2|N_1 = k_1) - P(N_2 = k_2)| \right\}. \end{aligned}$$

Let

$$\begin{aligned}
D_{k_1} &:= \sum_{k_2=0}^n \left( 1 + k_2^{\frac{q}{2}} + \frac{k_2^{\frac{q+l}{2}}}{\Delta^{\frac{l}{2}}} \right) |P(N_2 = k_2 | N_1 = k_1) - P(N_2 = k_2)| \\
&\leq \mathbb{E}_{N \sim B(n, \frac{1}{n_2})} \left( 1 + N^{\frac{q}{2}} + \frac{N^{\frac{q+l}{2}}}{\Delta^{\frac{l}{2}}} \right) + \mathbb{E}_{N \sim B(n-k_1, \frac{1}{n_2-1})} \left( 1 + N^{\frac{q}{2}} + \frac{N^{\frac{q+l}{2}}}{\Delta^{\frac{l}{2}}} \right) \\
&\leq \mathbb{E}_{N \sim B(n, \frac{1}{n_2})} \left( 1 + N^{\frac{q}{2}} + \frac{N^{\frac{q+l}{2}}}{\Delta^{\frac{l}{2}}} \right) + \mathbb{E}_{N \sim B(n, \frac{1}{n_2-1})} \left( 1 + N^{\frac{q}{2}} + \frac{N^{\frac{q+l}{2}}}{\Delta^{\frac{l}{2}}} \right) \\
&\leq C_{sup} \Delta^{\frac{q}{2}} + C_{sup} \left( \frac{n}{n_2-1} \right)^{\frac{q}{2}} + C_{sup} \left( \frac{n}{n_2-1} \right)^{\frac{q+l}{2}} \frac{1}{\Delta^{\frac{l}{2}}} \quad (\text{Lemma 2.13}) \\
&\leq C_{sup} \Delta^{\frac{q}{2}}.
\end{aligned}$$

Consider a fixed  $r \geq 0$ , to be specified later as a function of  $q$ . Then, by writing, as a convention for  $t \in \mathbb{R}$ ,  $\sum_{k=t}^n (\cdot)$  for  $\sum_{k=0, \dots, n; k \geq t} (\cdot)$ , we have

$$\begin{aligned}
\sum_{k_1=\Delta^r}^n \left( 1 + k_1^{\frac{q}{2}} + \frac{k_1^{\frac{q+l}{2}}}{\Delta^{\frac{l}{2}}} \right) P(N_1 = k_1) D_{k_1} &\leq C_{sup} \Delta^{\frac{q}{2}} \mathbb{E}_{N \sim B(n, \frac{1}{n_2})} \left( \mathbf{1}_{N \geq \Delta^r} \left[ N^{\frac{q}{2}} + \frac{N^{\frac{q+l}{2}}}{\Delta^{\frac{l}{2}}} \right] \right) \\
&(\text{Lemma 3.3}): \leq C_{sup} \Delta^{\frac{q}{2}} \left( \frac{\Delta^{\frac{q}{2}-1}}{\Delta^{2(r-1)}} + \frac{1}{\Delta^{\frac{l}{2}}} \frac{\Delta^{\frac{q+l}{2}-1}}{\Delta^{2(r-1)}} \right) \\
&\leq C_{sup} \Delta^{q-2r+1}. \tag{9}
\end{aligned}$$

We also have

$$\begin{aligned}
&\sup_{k_1 \leq \Delta^r} \sum_{k_2=\Delta^r}^n \left( 1 + k_2^{\frac{q}{2}} + \frac{k_2^{\frac{q+l}{2}}}{\Delta^{\frac{l}{2}}} \right) |P(N_2 = k_2 | N_1 = k_1) - P(N_2 = k_2)| \\
&\leq \sum_{k_2=\Delta^r}^n \left( 1 + k_2^{\frac{q}{2}} + \frac{k_2^{\frac{q+l}{2}}}{\Delta^{\frac{l}{2}}} \right) P(N_2 = k_2) + \sup_{k_1 \leq \Delta^r} \sum_{k_2=\Delta^r}^{n-k_1} \left( 1 + k_2^{\frac{q}{2}} + \frac{k_2^{\frac{q+l}{2}}}{\Delta^{\frac{l}{2}}} \right) P(N_2 = k_2 | N_1 = k_1) \\
&\leq C_{sup} \Delta^{\frac{q}{2}-2r+1} + \sup_{k_1 \leq \Delta^r} \mathbb{E}_{N \sim B(n-k_1, \frac{1}{n_2-1})} \left[ \mathbf{1}_{N \geq \Delta^r} \left( 1 + N^{\frac{q}{2}} + \frac{N^{\frac{q+l}{2}}}{\Delta^{\frac{l}{2}}} \right) \right] \quad (\text{from proof of (9)}) \\
&\leq C_{sup} \Delta^{\frac{q}{2}-2r+1} + \mathbb{E}_{N \sim B(n, \frac{2}{n_2})} \left[ \mathbf{1}_{N \geq \Delta^r} \left( 1 + N^{\frac{q}{2}} + \frac{N^{\frac{q+l}{2}}}{\Delta^{\frac{l}{2}}} \right) \right] \\
&\leq C_{sup} \Delta^{\frac{q}{2}-2r+1} + C_{sup} \frac{(2\Delta)^{\frac{q}{2}-1}}{\left( \frac{\Delta^{r-1}}{2} \right)^2} \quad (\text{from Lemma 3.3}) \\
&\leq C_{sup} \Delta^{\frac{q}{2}-2r+1}.
\end{aligned}$$

Hence, by writing, as a convention for  $t \in \mathbb{R}$ ,  $\sum_{k=0}^t (\cdot)$  for  $\sum_{k=0, \dots, n; k \leq t} (\cdot)$ , we have

$$\begin{aligned}
&\sum_{k_1=0}^{\Delta^r} \left( 1 + k_1^{\frac{q}{2}} + \frac{k_1^{\frac{q+l}{2}}}{\Delta^{\frac{l}{2}}} \right) P(N_1 = k_1) \left\{ \sum_{k_2=\Delta^r}^n \left( 1 + k_2^{\frac{q}{2}} + \frac{k_2^{\frac{q+l}{2}}}{\Delta^{\frac{l}{2}}} \right) |P(N_2 = k_2 | N_1 = k_1) - P(N_1 = k_1)| \right\} \\
&\leq C_{sup} \Delta^{\frac{q}{2}-2r+1} \sum_{k_1=0}^{\Delta^r} \left( 1 + k_1^{\frac{q}{2}} + \frac{k_1^{\frac{q+l}{2}}}{\Delta^{\frac{l}{2}}} \right) P(N_1 = k_1) \\
&\leq C_{sup} \Delta^{\frac{q}{2}-2r+1} \left( \Delta^{\frac{q}{2}} \right) \quad (\text{from Lemma 2.13}). \\
&= C_{sup} \Delta^{q-2r+1} \tag{10}
\end{aligned}$$

Hence (8), (9) and (10) we have

$$\begin{aligned} & \text{cov}(f_1(X), f_2(X)) \\ & \leq C_{sup} \sum_{k_1=0}^{\Delta^r} \sum_{k_2=0}^{\Delta^r} \left(1 + k_1^{\frac{q}{2}} + \frac{k_1^{\frac{q+l}{2}}}{\Delta^{\frac{l}{2}}}\right) \left(1 + k_2^{\frac{q}{2}} + \frac{k_2^{\frac{q+l}{2}}}{\Delta^{\frac{l}{2}}}\right) |P(N_1 = k_1, N_2 = k_2) - P(N_1 = k_1)P(N_2 = k_2)| \\ & \quad + C_{sup} \Delta^{q-2r+1}. \end{aligned} \tag{11}$$

Let  $q_{k_1, k_2} = P(N_2 = k_2 | N_1 = k_1) / P(N_2 = k_2)$ .

Then, we obtain from Lemma 2.11,

$$\begin{aligned} & q_{k_1, k_2} \\ & = \frac{(n - k_1)!(n - k_2)!}{n!(n - k_1 - k_2)!} \left(\frac{1}{\frac{n_2-1}{n_2}}\right)^{k_2} \left(1 - \frac{1}{n_2 - 1}\right)^{n-k_1-k_2} \left(\frac{1}{1 - \frac{1}{n_2}}\right)^{n-k_2} \\ & = \frac{(n - k_2)(n - k_2 - 1) \dots (n - k_2 - k_1 + 1)}{n(n - 1) \dots (n - k_1 + 1)} \left(\frac{n_2}{n_2 - 1}\right)^{k_2} \left(1 - \frac{1}{n_2 - 1}\right)^{n-k_1-k_2} \left(\frac{n_2}{n_2 - 1}\right)^{n-k_2} \\ & = \left(1 - \frac{k_2}{n}\right) \left(1 - \frac{k_2}{n-1}\right) \dots \left(1 - \frac{k_2}{n - k_1 + 1}\right) \left(1 + \frac{1}{n_2 - 1}\right)^{k_2} \left(1 - \frac{1}{n_2 - 1}\right)^{n-k_1-k_2} \left(1 + \frac{1}{n_2 - 1}\right)^{n-k_2} \\ & = \left(1 - \frac{k_2}{n}\right) \left(1 - \frac{k_2}{n-1}\right) \dots \left(1 - \frac{k_2}{n - k_1 + 1}\right) \left(1 + \frac{1}{n_2 - 1}\right)^{k_2} \left(1 - \frac{1}{n_2 - 1}\right)^{-k_1} \left(1 - \left[\frac{1}{n_2 - 1}\right]^2\right)^{n-k_2}. \end{aligned}$$

We now impose on  $r$  the condition  $\Delta^r = o(n)$ . Then since  $n, n_2 \rightarrow +\infty$ , we have for  $n$  large enough and  $k_1, k_2 \leq \Delta^r$ ,

$$\left(1 - 2\frac{\Delta^r}{n}\right)^{\Delta^r} \left(1 - \frac{2}{n_2^2}\right)^n - 1 \leq q_{k_1, k_2} - 1 \leq \left(1 + \frac{2}{n_2}\right)^{\Delta^r} \left(1 - \frac{2}{n_2}\right)^{-\Delta^r} - 1.$$

Let us add the condition on  $r$  that  $\Delta^{2r}/n$  and  $\Delta^r/n_2$  go to 0 as  $n \rightarrow \infty$ . Note also that the condition  $\Delta = O(n^{1/(2q+5)})$  implies  $n/n_2^2$  go to 0 as  $n \rightarrow \infty$ . Then one sees, by first using first-order Taylor expansions of the logarithms of the two products in the above display and then applying the exponential function, that there is a finite constant  $C_{sup}$ , independent of  $n$ , so that

$$|q_{k_1, k_2} - 1| \leq C_{sup} \left(\frac{\Delta^{2r}}{n} + \frac{n}{n_2^2} + \frac{\Delta^r}{n_2}\right). \tag{12}$$

Hence, from (11) and (12), we have

$$\begin{aligned} & \text{cov}(f_1(X), f_2(X)) \\ & \leq C_{sup} \sum_{k_1=0}^{\Delta^r} \sum_{k_2=0}^{\Delta^r} \left(1 + k_1^{\frac{q}{2}} + \frac{k_1^{\frac{q+l}{2}}}{\Delta^{\frac{l}{2}}}\right) \left(1 + k_2^{\frac{q}{2}} + \frac{k_2^{\frac{q+l}{2}}}{\Delta^{\frac{l}{2}}}\right) P(N_1 = k_1)P(N_2 = k_2) \left(\frac{\Delta^{2r}}{n} + \frac{n}{n_2^2} + \frac{\Delta^r}{n_2}\right) \\ & \quad + C_{sup} \Delta^{q-2r+1}. \\ & \leq C_{sup} \left(1 + \Delta^{\frac{q}{2}}\right)^2 \left(\frac{\Delta^{2r}}{n} + \frac{n}{n_2^2} + \frac{\Delta^r}{n_2}\right) + C_{sup} \Delta^{q-2r+1} \quad (\text{Lemma 2.13}) \\ & \leq C_{sup} \left(\frac{\Delta^{q+2r}}{n} + \frac{n\Delta^q}{n_2^2} + \frac{\Delta^{r+q}}{n_2} + \Delta^{q-2r+1}\right). \end{aligned} \tag{13}$$

Now, by choosing  $r = \frac{q}{2} + 2$  and by using the conditions  $\Delta \rightarrow +\infty$ , and  $\Delta = O(n^{1/(2q+5)})$  which implies, with a constant  $C_{inf} > 0$ ,  $n_2 \geq C_{inf} n^{(2q+4)/(2q+5)}$ , we check that the four terms of (13) converge to 0, and that the different conditions on  $r$  that we had imposed hold.  $\square$

*Proof of Lemma 2.13.* The lemma is true for  $k = 0$  and  $k = 1$ . Let  $B_1, \dots, B_n$  follow independently the Bernoulli  $(\frac{1}{n_2})$  distribution. Then, for  $k \geq 2$

$$\begin{aligned}
\mathbb{E} \left( \left[ \sum_{i=1}^n B_i \right]^k \right) &= n \mathbb{E} \left( B_1 \left[ \sum_{j=1}^n B_j \right]^{k-1} \right) \quad (\text{symmetry}) \\
&= \frac{n}{n_2} \mathbb{E} \left( \left[ 1 + \sum_{j=2}^n B_j \right]^{k-1} \right) \\
&\leq \Delta 2^{k-1} \mathbb{E} \left( 1 + \left[ \sum_{j=2}^n B_j \right]^{k-1} \right) \\
&\leq 2^{k-1} \Delta + 2^{k-1} \Delta \mathbb{E} \left( \left[ \sum_{j=1}^n B_j \right]^{k-1} \right).
\end{aligned}$$

This proves the lemma by induction on  $k$ . □

*Proof of Lemma 2.14.* Similar to the proof of Lemma D.1 in Bachoc (2014). □

*Proof of Lemma 2.15.* Each of the square component of  $Ab$  is the square of an inner product to which we can apply Cauchy-Schwarz inequality. Bounding the square of the Euclidean norms of the lines of  $A$  by  $m_2 \max_{i,j} A_{i,j}^2$  then gives the lemma. □

## References

- Adams, R. and Fournier, J. (2003). Sobolev spaces. Academic Press, Amsterdam.
- Bachoc, F. (2013). Cross validation and maximum likelihood estimations of hyper-parameters of Gaussian processes with model misspecification. Computational Statistics and Data Analysis, 66:55–69.
- Bachoc, F. (2014). Asymptotic analysis of the role of spatial sampling for covariance parameter estimation of gaussian processes. Journal of Multivariate Analysis, 125:1–35.
